# Supplementary material for: On the origin of the type-III radiation observed near the Sun
Source: arXiv:2403.05984 source file (2024-09-01)
Supplement: Supplementary file 1 [file Appendices.pdf]

# Appendices

**From July 2021, all appendices are published as camera-ready material.**

The success of the A&A journal brings with it a rapid growth in the number of articles and pages. As a consequence of this success and to keep down production costs, A&A will not typeset Appendices pages any longer but will include them at the end of the article as camera-ready material.

Appendices must be prepared even more carefully by the authors, because this part of the article will be published as camera-ready material, i.e., it will not be typeset by the Publisher. No correction, no copyediting, nor change of the layout in the appendices pages will be made in the LaTeX file after the receipt of the accepted version by the Publisher.

The following guide identifies the main layout issues we have identified, and how you can address them in the preparation of your Appendices in the LaTeX file:


- Placement of the Appendices at the end of the article
- Appendix sections
- Labels and citations
- Placement of illustrations (floats)
- Tables/figures longer than one page and/or wider than page width (landscape format)


## Placement of the Appendices at the end of the article

Appendices are included at the end of the article, after the reference list (or after the long list of affiliations if any, in the PDF file): they must begin on the next page of the PDF file.

In the .tex file, put appendices **after** `\end{thebibliography}`.

After compilation with the **new aa.cls** file for the A&A class, appendices will be placed automatically on a new page.

## Appendix sections

Put all the appendix sections into a single **environment "appendix"**. Then all sections that follow will be numbered with capital letters. Please do NOT use the "\appendix" command instead of the environment "appendix", for a better management of the counters of Figure/Table which can be placed at the end of the article.
